# Supplementary material for: Criticality and marginal stability of the shear jamming transition of frictionless soft spheres
Source: arXiv:2201.09726 ancillary file (2022-01-24)
Supplement: Supplementary file 1 [file SHEAR_JAMMING_SM.pdf]

# Supplemental Material of “Criticality and marginal stability of the shear jamming transition of frictionless soft spheres”

Additional material supporting the results in the main text are organised here as follows: In Sec. I we provide details of the iterative procedure to generate configurations with a single self-stressed state. In Sec. II we provide details of the computation of the Hessian and the stiffness matrix. In Sec. III we show the fabric anisotropy of shear jammed configurations at different  $\phi$ . In Sec. IV we show results for pressure and contact number for 2D and 3D. In Sec. V we show size dependence of the shear jamming line *vs.* density, and results concerning the finite size scaling of the gap distribution.

## I. ITERATIVE PROCEDURE TO GENERATE CONFIGURATIONS WITH SINGLE SELF-STRESSED STATES ( $N_{SS} = 1$ )

The potential energy  $U$  scales with respect to the distance from the jamming strain  $\gamma_j$  as

$$U \propto (\gamma - \gamma_j)^2 \quad (1)$$

This dependence is shown in fig.1 for two and three dimensions.

If we assume that we know the value of  $\gamma_j$ , and start with an initial jammed configuration at  $\gamma_0 > \gamma_j$ , we can generate  $n$  logarithmically placed configurations between  $\gamma_0$  and  $\gamma_j + (\gamma_0 - \gamma_j) \times 10^{-1}$  using the iteration

$$\begin{aligned} \log(\gamma_{i+1} - \gamma_j) - \log(\gamma_i - \gamma_j) &= -\frac{1}{n} \\ \gamma_{i+1} &= \gamma_j + (\gamma_i - \gamma_j) \times 10^{-\frac{1}{n}} \end{aligned} \quad (2)$$

However, we do not know the precise value of  $\gamma_j$ , but can iteratively approximate  $\gamma_j$  as well. From Eq. 1 we have

$$\begin{aligned} \sqrt{\frac{U_{i+1}}{U_i}} &= \frac{\gamma_{i+1} - \gamma_j}{\gamma_i - \gamma_j} \\ \gamma_j &= \frac{\gamma_{i+1} - \gamma_i \times \sqrt{\frac{U_{i+1}}{U_i}}}{\left(1 - \sqrt{\frac{U_{i+1}}{U_i}}\right)} \end{aligned} \quad (3)$$

If we calculate a new strain  $\gamma_{i+1}$  using Eq. 2 and use that strain to calculate a new jamming strain using Eq. 3, then we have an iterative procedure to approximate  $\gamma_j$  better and also find configurations close to it. With  $\tilde{\gamma}_i$  being the jamming strain estimated at the  $i$ 'th iteration, we have

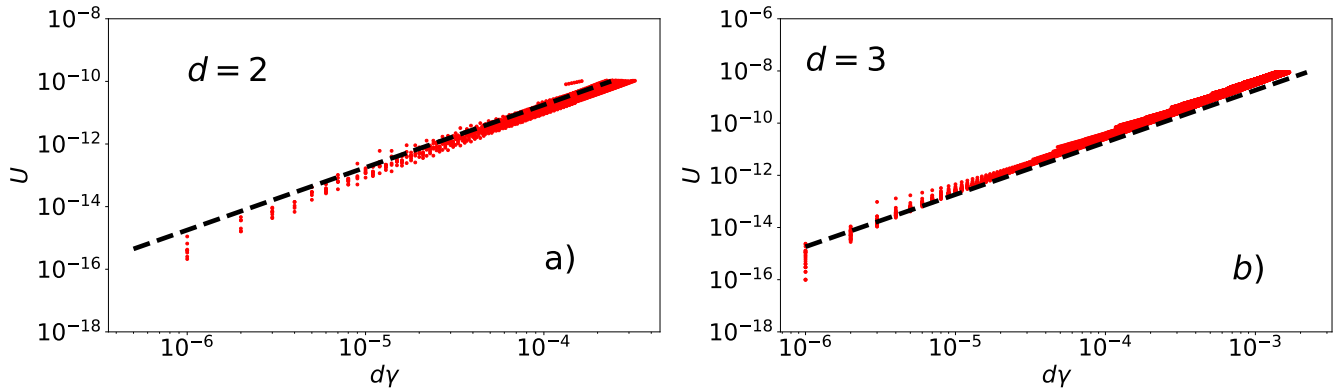

FIG. 1: Evolution of potential energy  $U$  during the final reverse shear from the SJ procedure.  $U \sim d\gamma^2$ , this information is used in IP to go closer to  $\gamma_j$  for **a)**  $d = 2$  **b)**  $d = 3$

$$\gamma_{i+1} = \tilde{\gamma}_i + (\gamma_i - \tilde{\gamma}_i) \times 10^{-\frac{1}{n}} \quad (4)$$

$$\tilde{\gamma}_{i+1} = \frac{\gamma_{i+1} - \gamma_i \times \sqrt{\frac{U_{i+1}}{U_i}}}{\left(1 - \sqrt{\frac{U_{i+1}}{U_i}}\right)} \quad (5)$$

Configurations generated using this procedure are analyzed by removing the rattlers recursively. After removing the rattlers if the configurations satisfies  $N_c = (N - 1)d + 1$  then the configuration has only one self-stressed state and we use it for the force and gap distribution analysis, while others are discarded.

This procedure is adopted from Charbonneau et al [1] where it is described for isotropic jamming.

## II. HESSIAN AND THE STIFFNESS MATRIX

In a  $d = 3$  system we have a total of 6 independent strain direction represented as  $\eta_{xx}, \eta_{yy}, \eta_{zz}, \eta_{xz}, \eta_{yz}, \eta_{xy}$ . Deforming the system costs energy and all deformations are a linear sum of these strains. We define therefore the matrix of elastic constants.

$$C_{\alpha\beta\gamma\sigma} = \frac{1}{V} \frac{d^2 U}{d\eta_{\alpha\beta} d\eta_{\gamma\sigma}}$$

or the stiffness matrix. The elastic constants for a configuration at mechanical equilibrium is given by [2]

$$C_{\alpha\beta\kappa\lambda} = \frac{1}{V} \frac{\partial U}{\partial \eta_{\alpha\beta} \partial \eta_{\kappa\lambda}} + \frac{1}{V} \sum_{ij, \chi\delta} \Xi_{\alpha\beta}^{i\chi} (\mathbf{H}^{-1})_{ij}^{\chi\delta} \Xi_{\kappa\lambda}^{j\delta} \quad (6)$$

where

$$\mathbf{H}_{ij}^{\alpha\beta} = \frac{\partial^2 U}{\partial r_{i\alpha} \partial r_{j\beta}}$$

is the Hessian and

$$\Xi_{\kappa\lambda}^{i\alpha} = - \frac{\partial^2 U}{\partial r_{i\alpha} \partial \eta_{\kappa\lambda}}$$

In Eq. 6 the first term represents the contribution to elastic constant due to the affine displacement of the particles. The second term can be understood as follows. During AQS shear protocol, the first step is the affine transformation of the particle co-ordinates according to the strain applied. After this affine transformation there will be forces which are unbalanced, give rise to the non-affine displacement field of the particles. The contribution of these non-affine displacements is the second term of Eq. 6.

For a system of particles interacting *via* a pair-wise potential, the expression for  $C_{\alpha\beta\kappa\lambda}$  above can be evaluated as follows. Defining

$$t_{ij} = \frac{\partial u(r_{ij})}{\partial r_{ij}}; c_{ij} = \frac{\partial^2 u(r_{ij})}{\partial r_{ij}^2}$$

we have

$$\Xi_{\kappa\lambda}^{i\alpha} = - \sum_j (r_{ij} c_{ij} - t_{ij}) \eta_{ij}^\alpha \eta_{ij}^\kappa \eta_{ij}^\lambda \quad (7)$$

and

$$\frac{\partial U}{\partial \eta_{\alpha\beta} \partial \eta_{\kappa\lambda}} = \frac{1}{V} \sum_{ij} (r_{ij} c_{ij} - t_{ij}) r_{ij} \eta_{ij}^\alpha \eta_{ij}^\beta \eta_{ij}^\kappa \eta_{ij}^\lambda \quad (8)$$

where  $r_{ij}$  is the distance between the centers of particles that are in contact and  $\hat{n}_{ij}$  is the unit vector connecting the centers of the two particles.

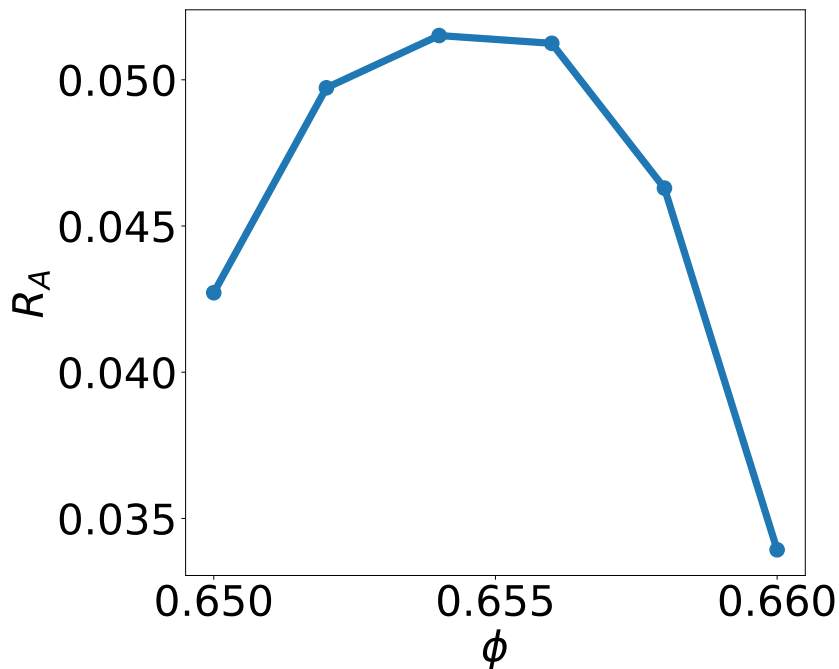

FIG. 2: Fabric anisotropy  $R_A$  of shear jammed configurations at different densities above  $\phi_J$ . The anisotropy shows a non-monotonic behavior similar to the projection of the strain vector on the stiffest eigen-vector of the stiffness matrix.

Using Eq. 7 and Eq. 8 in Eq. 6 and using the eigenvectors of the Hessian we can calculate the elastic constants. Derivation of equation(6) and other details can be found in [2].

After calculating the stiffness matrix, we diagonalize the matrix to get the eigenvalues and eigenvectors. It is observed that close to the jamming strain some eigen-values take negative values. As discussed in [3] the procedures used to generate jammed configurations does not guarantee that the configurations are stable against any strain perturbation. Therefore these configurations generally can have negative eigenvalues for the stiffness matrix. In calculating the scaling of eigenvalues near jamming, we discard configurations for which any of the eigenvalues are negative. We have compared the values of the stiffness matrix elements obtained using Eq. 6 with the values obtained through a finite difference formula and have confirmed that consistent results are obtained.

### III. FABRIC ANISOTROPY

The fabric tensor is defined as

$$\mathbf{F} = \frac{1}{V} \sum_{i < j} \frac{\vec{r}_{ij}}{|\vec{r}_{ij}|} \otimes \frac{\vec{r}_{ij}}{|\vec{r}_{ij}|}$$

This is analogous to the stress tensor and one can compute the eigenvalues of this tensor. The fabric anisotropy is defined as

$$R_A = \frac{\lambda_1 - \lambda_3}{\lambda_1 + \lambda_2 + \lambda_3}$$

where the  $\lambda_1 > \lambda_2 > \lambda_3$ . The fabric anisotropy being zero implies that no direction in space is special and therefore the system is iso-tropic. The anisotropy of the configurations that are shear jammed at different densities is shown in Fig.2.  $R_A$  has a non-monotonic behavior and it approaches zero as we shear jam configurations close to the isotropic jamming density  $\phi_J$ .

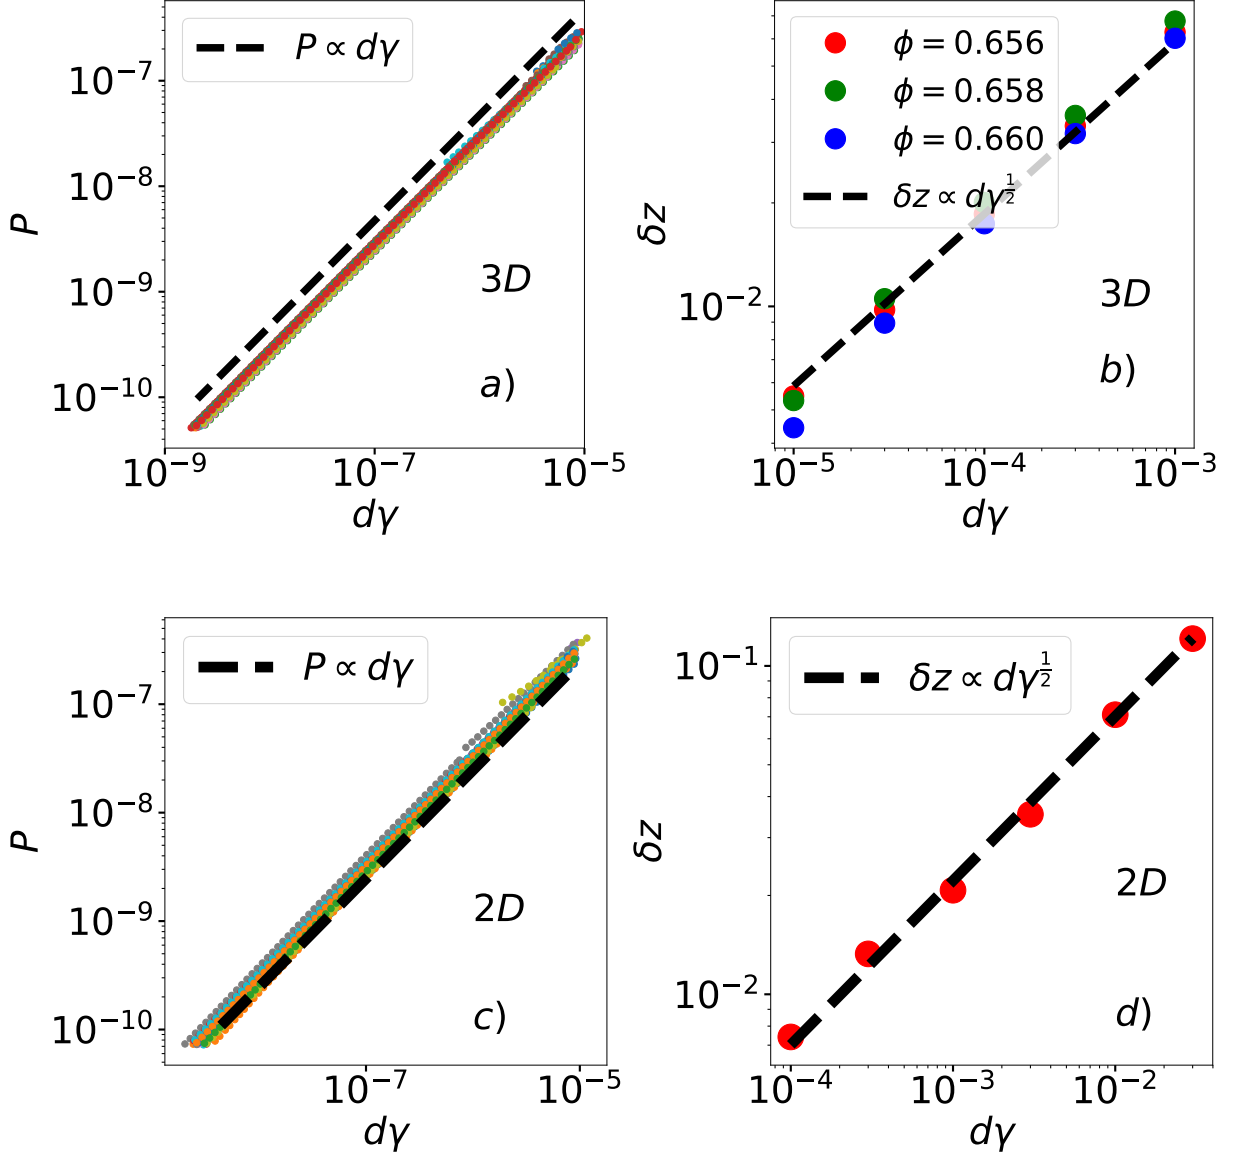

FIG. 3: Scaling near the shear jamming transition for 3D and 2D soft-spheres **a)** Pressure  $P \sim d\gamma$ . Data is from the iterative procedure IP. Data from individual runs are shown. **b)** Excess contact number  $\delta z \sim d\gamma^{\frac{1}{2}}$ . **c)** and **d)** are the corresponding results in 2D. In **c)**, **d)** the density is 0.8499.

#### IV. PRESSURE AND CONTACT NUMBER IN 3D AND 2D

Using the same methods described in the main draft we generate shear jammed configurations for 2D system. For 2D system the value of  $\phi_j$  we generate is approximately 0.851. We generate the configurations at  $\phi_j \approx 0.851$  and decompress the configurations to densities  $\phi$  such that  $\phi_j < \phi < \phi_j$ . Shear jammed configurations with a single self-stressed states are generated in the same way as described in the main text. Below we present the scaling of the pressure and the excess contact number for two and three dimensional systems near shear jamming.

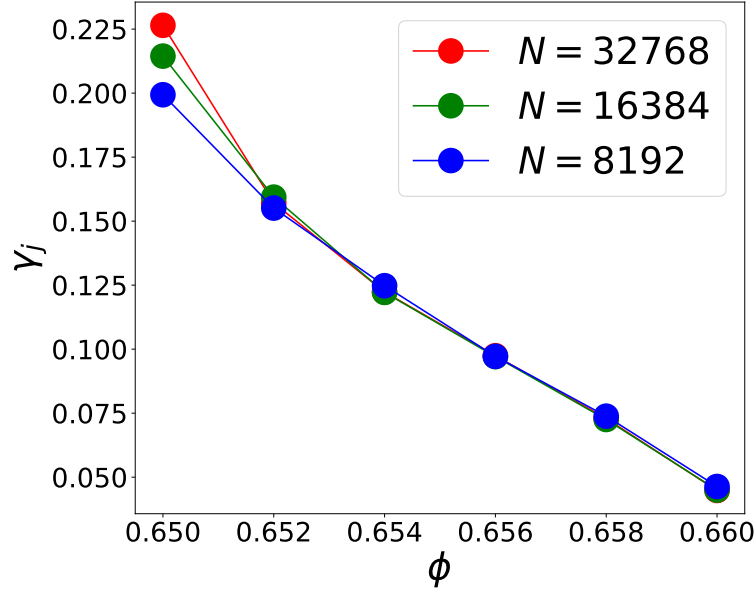

FIG. 4: Dependence of  $\gamma_j$  on the density of the system  $\phi$  shown for various system sizes.

#### V. SYSTEM SIZE DEPENDENCE OF THE JAMMING STRAIN AND FINITE SIZE SCALING OF THE GAP DISTRIBUTION

The dependence of the jamming strain on the system size is shown in Fig. 4. Configurations at the isotropic jamming density  $\phi_j \approx 0.66$  are generated for  $N = 2^{12}, 2^{13}, 2^{14}, 2^{15}$  and are decompressed to densities such that  $\phi_J < \phi < \phi_j$ . These configurations are sheared uniformly to observe shear jamming at some strain  $\gamma_j(\phi)$ . Although we observe weak size dependence at the lowest densities, close to  $\phi_J$  (as also in [4]), for most of the range of densities, we do not observe any significant size effects.

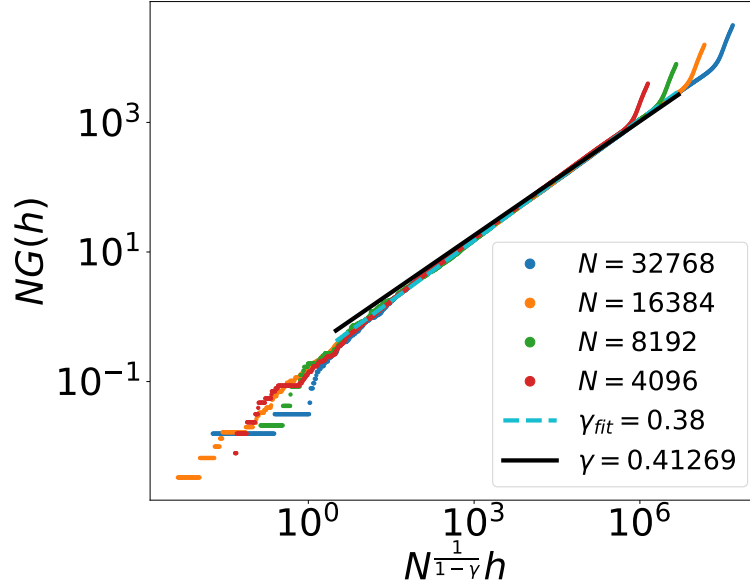

FIG. 5: Finite size scaling of gap distribution  $G(h)$  demonstrating that the mean field exponent of  $\gamma = 0.41269$  convincingly fits the data in the region of data collapse. Also shown is a fit with  $\gamma_{fit} = 0.38$  for comparison.

We analyze the gap distribution  $G(h)$  obtained from different system sizes. We use the finite size scaling form given

in [5]  $c(h) \sim N^{-1}\tilde{c}(hN^{\frac{1}{1-\gamma}})$ , employing the mean field value of the exponent  $\gamma$ . The results in Fig. 5 show convincing data collapse, with the data in the collapsed region being extremely well described by the mean field  $\gamma$  value. A smaller  $\gamma_{fit}$  value of 0.38 also describes the data reasonably well, but from the data collapse, one may conclude that such a fit is affected by the finite size deviations at small  $x$  values.

- 
- [1] P. Charbonneau, E. I. Corwin, G. Parisi, and F. Zamponi, Jamming criticality revealed by removing localized buckling excitations, *Physical review letters* **114**, 125504 (2015).
  - [2] A. Lemaître and C. Maloney, Sum rules for the quasi-static and visco-elastic response of disordered solids at zero temperature, *Journal of statistical physics* **123**, 415 (2006).
  - [3] C. P. Goodrich, S. Dagois-Bohy, B. P. Tighe, M. Van Hecke, A. J. Liu, and S. R. Nagel, Jamming in finite systems: Stability, anisotropy, fluctuations, and scaling, *Physical Review E* **90**, 022138 (2014).
  - [4] Y. Jin and H. Yoshino, A jamming plane of sphere packings, *Proceedings of the National Academy of Sciences* **118** (2021).
  - [5] P. Charbonneau, E. I. Corwin, R. C. Dennis, R. D. H. Rojas, H. Ikeda, G. Parisi, and F. Ricci-Tersenghi, Finite-size effects in the microscopic critical properties of jammed configurations: A comprehensive study of the effects of different types of disorder, *Physical Review E* **104**, 014102 (2021).
